# Supplementary material for: Silver electrodes are highly selective for CO in CO$_2$ electroreduction due to interplay between voltage dependent kinetics and thermodynamics
Source: arXiv:2408.15124 ancillary file (2025-12-17)
Supplement: Supplementary file 1 [file supporting_info.pdf]

# Supporting Information: Silver electrodes are highly selective for CO in $CO_2$ electroreduction due to interplay between voltage dependent kinetics and thermodynamics

Michele Re Fiorentin,[†,§] Francesca Risplendi,[†,§] Clara Salvini,[†] Juqin Zeng,[†]

Giancarlo Cicero,[†] and Hannes Jónsson[*,‡,¶]

†*Department of Applied Science and Technology, Politecnico di Torino, corso Duca degli Abruzzi 24, 10129 Torino, Italy*

‡*Science Institute and Faculty of Physical Sciences, University of Iceland, 107 Reykjavík, Iceland*

¶*Department of Chemistry, Brown University, Providence, Rhode Island 02912, United States*

§*These authors contributed equally to this work.*

E-mail: hj@hi.is

## Computational Details

### DFT setup

Theoretical calculations rely on DFT electronic structure calculations coupled with an implicit solvation model, implemented in the VASP[?,?,?,?] and VASPsol[?,?,?] packages. This allows for describing the system under specific applied voltages, aiding in the identification

of reaction mechanisms and accurate estimation of transition state energies in electrochemical reduction processes. Specifically, the Kohn-Sham equations[?] were solved using ultrasoft pseudopotential to describe the electron-ion interaction, employing the revised gradient-corrected Perdew-Burke- Ernzerhof (rPBE) functional[?] to describe the exchange-correlation effects, the projector augmented wave (PAW) pseudopotential with a cutoff energy of 350 eV was adopted to describe the core electrons for H, C, O, and Ag (valence of $4d^{10}$ and $5s^1$).[?] The Ag surfaces, (111), (100), and (110), were modeled using, respectively, c(3×4), p(3×3), and p(2×4) supercells, each comprising a silver slab with four atomic layers. (4×3×1), (4×4×1), and (4×3×1) Monkhorst-Pack grids were employed for Brillouin zone integration.[? ?] A vacuum region of 10 Å thickness was added in the cells to avoid spurious interaction between periodic replicas along the surface orthogonal direction. All structures were relaxed by minimizing the atomic forces and convergence was assumed when the maximum component of the residual forces on the ions is smaller than 0.05 eV/Å. In all calculations, the bottom two layers were fixed, while the topmost layers were allowed to relax.

## Thermodynamics and kinetics

The thermodynamic study was carried out adopting the thermochemical model (TCM).[? ? ?] For the calculation of the entropic corrections to adsorbates, all degrees of freedom were considered as vibrational and treated in the harmonic approximation. The chemical potentials of gas species ($H_2$, $CO_2$ and CO) were obtained following standard ideal-gas methods. To account for the systematic error introduced by the RPBE functional in the energetics of C=O bonds, corrections of -0.07 eV and -0.46 eV were applied to the electronic energy of the CO and $CO_2$ molecules, respectively.[?] The chemical potentials of liquid or solvated species were derived from the computed gas-phase potentials and corrected with thermochemical data.

Transition states (TSs) were identified by performing a nudged elastic band (NEB) calculation starting from the relaxed initial state (IS). The TS was then optimized at constant

potential with the dimer method. Activation grand-canonical energies at constant potential $U$ are computed as $\Delta\Omega^{\ddagger}(U) = \Omega_{\mathrm{TS}}(U) - \Omega_{\mathrm{IS}}(U)$. The TS grand-canonical free energy $G_{\mathrm{TS}}$ can be obtaned from $\Omega_{\mathrm{TS}}$ by including the zero-point energy and entropic contributions obtained from the TS vibrational modes, excluding the imaginary one. To correctly reference activation grand-canonical free energies to solvated $H_3O^+$ ions in the electrolyte bulk, instead of relying on the ISs used in the TS search, we computed the grand-canonical free energies $G_{\mathrm{IS}}$ using the TCM. Similarly, solvated molecules, such as $CO_2$ were treated thermochemically.[?]

## Reaction Mechanisms

In our investigation, we focused on $CO_2$ conversion towards CO and HCOOH can be achieved by two proton-electron transfers.

Here, the two pathways that we kinetically investigate are the Tafel and the Heyrovsky mechanisms. In the Tafel mechanism, the $CO_2$RR intermediate is obtained from the reaction between a $CO_2$ molecule and a hydrogen atom $^*$H already adsorbed on the surface, as:

$$\mathrm{CO_2} +^* \mathrm{H} \longrightarrow {}^*\mathrm{COOH} \tag{1}$$

for $^*$COOH and a related mechanism, a Tafel-like mechanism, involves concerted H atom and electron transfer to $CO_2$ for $HCOO^-$ production, as:

$$\mathrm{CO_2} + \mathrm{e^-} +^* \mathrm{H} \longrightarrow \mathrm{HCOO^-} \tag{2}$$

The Heyrovsky mechanism firstly proceeds through the formation of either $^*$COOH or $^*$OCHO, in which the proton comes from the electrolyte. We consider hydronium ions ($H_3O^+$) as the proton source, so that we have:

$$\mathrm{CO_2} + \mathrm{H_3O^+} + \mathrm{e^-} + {}^* \longrightarrow {}^*\mathrm{COOH} + \mathrm{H_2O} \tag{3}$$

$$CO_2 + H_3O^+ + e^- + {}^* \longrightarrow {}^*OCHO + H_2O \tag{4}$$

The second proton electron transfer (PET) occuring after Eq. (4) only releases formate, as:

$$^*OCHO + H_3O^+ + e^- \longrightarrow HCOOH + 2\,H_2O + {}^* \tag{5}$$

$^*COOH$, instead, can react to form both HCOOH and CO. Therefore, a second Heyrovsky-like PET may occur either as:

$$^*COOH + H_3O^+ + e^- \longrightarrow CO + 2\,H_2O + {}^*, \tag{6}$$

or

$$^*COOH + H_3O^+ + e^- \longrightarrow HCOOH + H_2O + {}^*. \tag{7}$$

In addition, since the Tafel-like mechanism requires a hydrogen atom adsorbed on the metal surface, the Volmer-Heyrovsky mechanism for the HER was also considered.This pathway of HER unfolds as:

$$H_3O^+ + e^- + {}^* \longrightarrow {}^*H + H_2O, \tag{8}$$

$$^*H + H_3O^+ + e^- \longrightarrow H_2 + H_2O + {}^*, \tag{9}$$

where the $H^+$ is transferred from an $H_3O^+$ in solution to the surface.

Depending on the mechanism involved, the reaction pathway passes through a specific transition state (TS). This TS corresponds to a first-order saddle point of the energy surface, and determines the magnitude of the kinetic barrier ($\Delta\Omega_{\mathrm{act}}$). For HER, we introduce the TSs in the reactions steps Eqs. (8) and (9) as:

$$\underset{\text{initial}\,^{\text{Vol}}_{\text{HER}}}{H_3O^+ + e^- + {}^*} \longrightarrow \underset{\text{TS}\,^{\text{Vol}}_{\text{HER}}}{[\,^* \cdot\cdot H \cdot\cdot OH_2]} \longrightarrow \underset{\text{final}\,^{\text{Vol}}_{\text{HER}}}{^*H + H_2O} \tag{10}$$

for the first Volmer step, and

$$\underset{\text{initial}\,^{\text{Hey}}_{\text{HER}}}{{}^{*}\mathrm{H} + \mathrm{H_3O^+} + \mathrm{e^-}} \longrightarrow \underset{\text{TS}\,^{\text{Hey}}_{\text{HER}}}{[\,{}^{*}\mathrm{H}\cdot\cdot\mathrm{H}\cdot\cdot\mathrm{OH_2}]} \longrightarrow \underset{\text{final}\,^{\text{Hey}}_{\text{HER}}}{\mathrm{H_2} + \mathrm{H_2O} + \,{}^{*}} \tag{11}$$

for the second, Heyrovsky, step. Turning to $CO_2$RR, in the first step, reduced $CO_2$ can be adsorbed on the electrode surface either as *COOH:

$$\underset{\text{initial}\,^{\text{Hey}}_{\mathrm{CO_2}}}{\mathrm{CO_2} + \mathrm{H_3O^+} + \mathrm{e^-} + \,{}^{*}} \longrightarrow \underset{\text{TS}\,^{\text{Hey}}_{\mathrm{CO_2}\to\,{}^{*}\mathrm{COOH}}}{[\,{}^{*}\mathrm{CO_2}\cdot\cdot\mathrm{H}\cdot\cdot\mathrm{OH_2}]} \longrightarrow \underset{\text{final}\,^{\text{Hey}}_{{}^{*}\mathrm{COOH}}}{{}^{*}\mathrm{COOH} + \mathrm{H_2O}} \tag{12}$$

or HCOO*

$$\underset{\text{initial}\,^{\text{Hey}}_{\mathrm{CO_2}}}{\mathrm{CO_2} + \mathrm{H_3O^+} + \mathrm{e^-} + \,{}^{*}} \longrightarrow \underset{\text{TS}\,^{\text{Hey}}_{\mathrm{CO_2}\to\,\mathrm{HCOO^*}}}{[\,{}^{*}\mathrm{CO_2}\cdot\cdot\mathrm{H}\cdot\cdot\mathrm{OH_2}]} \longrightarrow \underset{\text{final}\,^{\text{Hey}}_{\mathrm{HCOO^*}}}{\mathrm{HCOO^*} + \mathrm{H_2O}} \tag{13}$$

The reduction step of the *COOH intermediate to CO can be written as:

$$\underset{\text{initial}\,^{\text{Hey}}_{{}^{*}\mathrm{COOH}}}{{}^{*}\mathrm{COOH} + \mathrm{H_3O^+} + \mathrm{e^-} + \,{}^{*}} \longrightarrow \underset{\text{TS}\,^{\text{Hey}}_{{}^{*}\mathrm{COOH}\to\,\mathrm{CO}}}{[\,{}^{*}\mathrm{CO_2H}\cdot\cdot\mathrm{H}\cdot\cdot\mathrm{OH_2}]} \longrightarrow \underset{\text{final}\,^{\text{Hey}}_{{}^{*}\mathrm{COOH}}}{\mathrm{CO} + 2\mathrm{H_2O} + \,{}^{*}} \tag{14}$$

and to HCOOH as:

$$\underset{\text{initial}\,^{\text{Hey}}_{{}^{*}\mathrm{COOH}}}{{}^{*}\mathrm{COOH} + \mathrm{H_3O^+} + \mathrm{e^-} + \,{}^{*}} \longrightarrow \underset{\text{TS}\,^{\text{Hey}}_{{}^{*}\mathrm{COOH}\to\,\mathrm{HCOOH}}}{[\,{}^{*}\mathrm{COOH}\cdot\cdot\mathrm{H}\cdot\cdot\mathrm{OH_2}]} \longrightarrow \underset{\text{final}\,^{\text{Hey}}_{\mathrm{HCOOH}}}{\mathrm{HCOOH} + \mathrm{H_2O} + \,{}^{*}}. \tag{15}$$

The reduction step of HCOO* leads to HCOOH as:

$$\underset{\text{initial}\,^{\text{Hey}}_{\mathrm{HCOO^*}}}{\mathrm{HCOO^*} + \mathrm{H_3O^+} + \mathrm{e^-} + \,{}^{*}} \longrightarrow \underset{\text{TS}\,^{\text{Hey}}_{\mathrm{HCOO^*}\to\,\mathrm{HCOOH}}}{[\mathrm{HCOO^*}\cdot\cdot\mathrm{H}\cdot\cdot\mathrm{OH_2}]} \longrightarrow \underset{\text{final}\,^{\text{Hey}}_{\mathrm{HCOOH}}}{\mathrm{HCOOH} + \mathrm{H_2O} + \,{}^{*}}. \tag{16}$$

Finally, assuming that a hydrogen atom is already adsorbed on the metal surface, the

first step of $CO_2$RR may be Tafel-like and proceed as either:

$$\underset{\text{initial }^{\text{Taf}}_{\text{CO}_2}}{{}^*\text{H} + \text{CO}_2 + {}^*} \longrightarrow \underset{\text{TS }^{\text{Taf}}_{\text{CO}_2 \rightarrow {}^*\text{COOH}}}{[\,{}^*\text{H} \cdot \cdot \text{CO}_2]} \longrightarrow \underset{\text{final }^{\text{Taf}}_{{}^*\text{COOH}}}{{}^*\text{COOH} + {}^*} \tag{17}$$

or

$$\underset{\text{initial }^{\text{Taf}}_{\text{CO}_2}}{{}^*\text{H} + \text{CO}_2 + \text{e}^- + {}^*} \longrightarrow \underset{\text{TS }^{\text{Taf}}_{\text{CO}_2 \rightarrow \text{HCOO}^-}}{[\,{}^*\text{H} \cdot \cdot \text{CO}_2]} \longrightarrow \underset{\text{final }^{\text{Taf}}_{\text{HCOO}^-}}{\text{HCOO}^- + {}^*} \tag{18}$$

# Transition State geometries

TS geometries for key steps in HER and $CO_2$RR are shown in Figure 1 for the prototype Ag(111) surface. These TS geometries were evaluated at $U = -1.5$ V vs. SHE, with similar structures observed at $U = -0.8$, $-1.2$, and $-1.8$ V vs SHE. Negligible differences were found, across these potentials, on different surfaces, including Ag(100) and Ag(110). The geometries were calculated using NEB and dimer methods.

# Experimental procedure

## Preparation of the Ag electrode

The Ag gas diffusion electrode (GDE) was prepared by sputter coating (Quorum Technologies Ltd Q150T). A carbon paper (GDL; SIGRACET 28BC, Ion Power GmbH) was used as the substrate and a silver disc (99.99%, Testbourne) as the target. The deposition was carried out at 50 mA for 200 seconds to obtain a Ag mass loading of about 151.3 $\mu$g cm$^{-2}$.

## Electrochemical tests and product analysis

The $CO_2$RR experiments were conducted in galvanostatic mode with a CHI760D potentiostat in a customized flow cell, as shown in Figure 2. Both catholyte and anolyte were a solution of pH 2, which was prepared by tuning 1.0 M KOH with concentrated $H_2SO_4$. A cation exchange

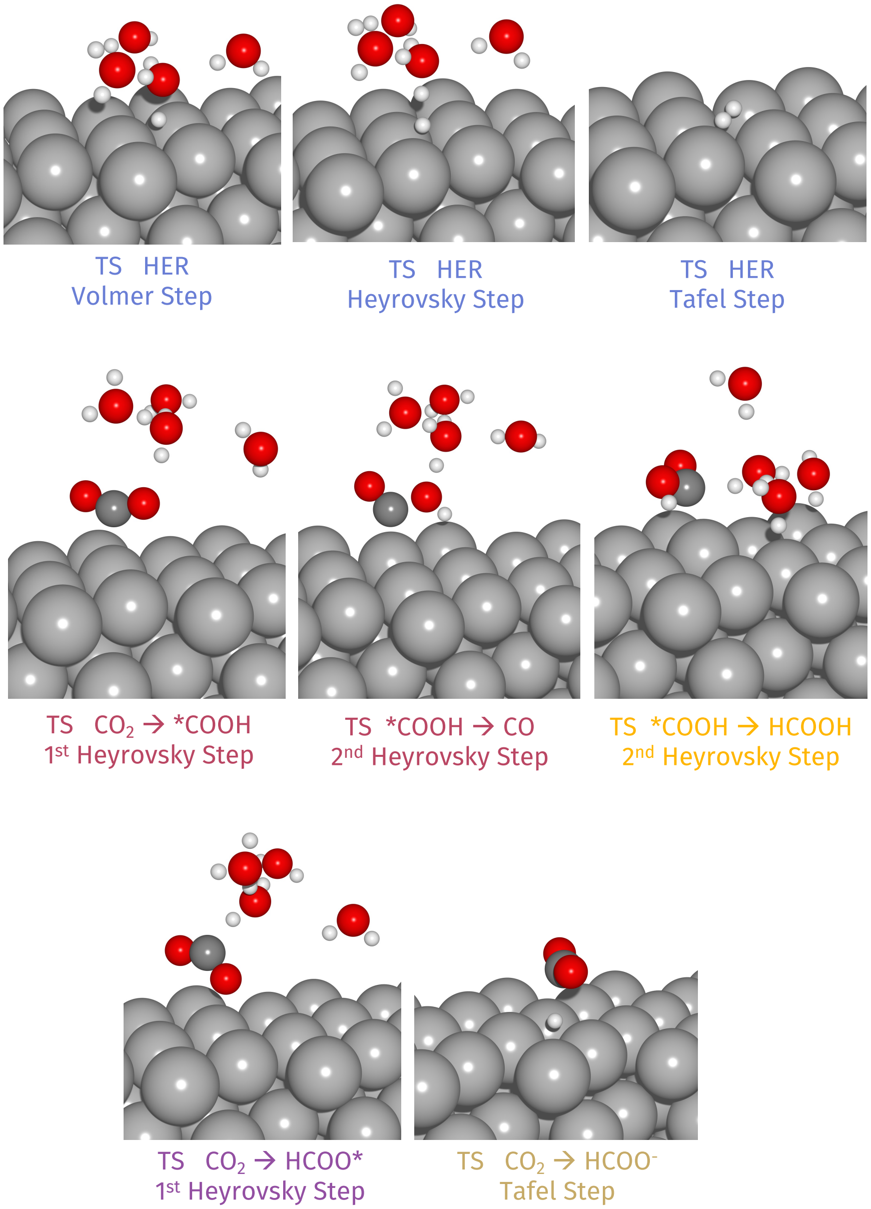


Figure 1: Geometries of transition states (TSs) for the different electrocatalytic reactions considered in this study on Ag(111) at $U = -1.5$ V vs. SHE. The top panels show HER TSs: Volmer (left), Heyrovsky (middle), and Tafel (right). The middle panels report $CO_2$RR TSs: the first Heyrovsky step for $CO_2$ to *COOH (left), the second step from *COOH to CO (middle), and the alternative pathway from *COOH to HCOOH (right). The bottom panels represent the first Heyrovsky step for $CO_2$ to HCOO* (left) and the Tafel step from CO2 to $HCCO^-$ (right). Each reaction is referenced below its respective figure, with colors corresponding to those used in Figure 2 of the manuscript.

membrane (Nafion™ membrane N117) was used to separate the cathodic and anodic sides.

The cathodic side was divided into two compartments by the working electrode, which is the Ag GDE with a geometric area of 1.5 $cm^2$. A mini Ag/AgCl (1 mm, leak-free LF-1) was inserted in the catholyte and used as the reference electrode. An Ir-coated Ti plate (Ir-MMO, 10 $cm^2$, ElectroCell Europe A/S) was immersed in the anolyte and used as the counter electrode. Both catholyte and anolyte were circuited at 4 mL min-1 during the test. A constant CO2 flow of 25 mL $min^{-1}$ was maintained at cathodic gas compartment. Electrode potentials were rescaled to the RHE scale by applying Nernst equation. Gas-phase products were analyzed on-line by a micro gas chromatograph (GC, Fusion®, INFICON), which is composed of two channels with a 10 m Rt-Molsieve 5A column and an 8 m Rt-Q-Bond column, respectively, and each channel with a micro thermal conductivity detector. The faradaic efficiency (FE) for each gas-phase product was determined from its concentration in the outlet gas stream, as

$$\mathrm{FE} = \frac{V\,t\,C\,n\,F}{V_m\,Q},$$

where $V_m$ is the molar volume of an ideal gas (L $mol^{-1}$); $V$ is the flow rate of $CO_2$ at the cathodic side (L $min^{-1}$); $t$ is electrolysis time (min); $Q$ is the total charge passed through the system during the electrolysis time $t$ (coulomb, C); $C$ is the concentration of the gas product (% v/v); $n$ is the number of electrons required to obtain 1 molecule of this product ($n = 2$ for CO and $H_2$ formation); $F$ is Faraday's constant (96485 C $mol^{-1}$). For the detection and quantification of liquid-phase products, a high-performance liquid chromatograph (HPLC, Thermo Scientific, Ultimate3000) was utilized. This HPLC system featured a UV-Vis detector set at a wavelength of 210 nm and a ReproGel chromatographic column with dimensions of 300 × 8 mm. The mobile phase used for the HPLC analysis was an aqueous solution of 9.0 mM $H_2SO_4$ delivered at a flow rate of 1.0 mL $min^{-1}$. The FE for each liquid product can be calculated from its concentration in the sampled catholyte as

$$\mathrm{FE} = \frac{v\,C\,n\,F}{Q},$$

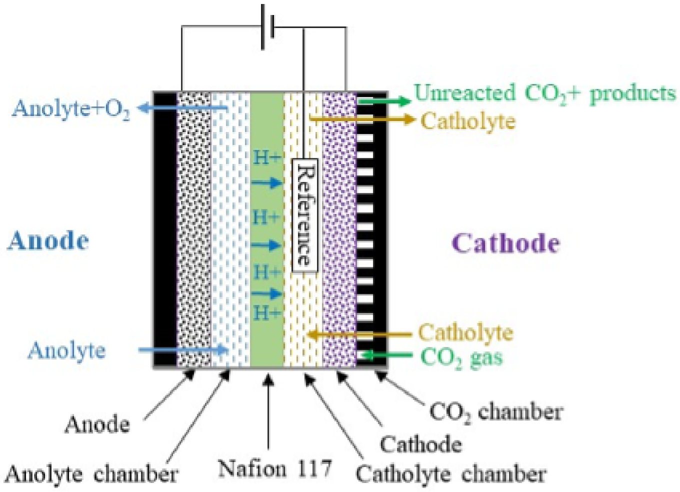


Figure 2: The scheme of the customized three-electrode three-compartment flow cell.

where $v$ is the volume of catholyte (L).

## References

() Kresse, G.; Hafner, J. Ab initio molecular dynamics for liquid metals. *Phys. Rev. B* **1993**, *47*, 558–561.

() Kresse, G.; Hafner, J. Ab initio molecular-dynamics simulation of the liquid-metal–amorphous-semiconductor transition in germanium. *Phys. Rev. B* **1994**, *49*, 14251–14269.

() Kresse, G.; Furthmüller, J. Efficiency of ab-initio total energy calculations for metals and semiconductors using a plane-wave basis set. *Computational Materials Science* **1996**, *6*, 15–50.

() Kresse, G.; Furthmüller, J. Efficient iterative schemes for ab initio total-energy calculations using a plane-wave basis set. *Phys. Rev. B* **1996**, *54*, 11169–11186.

() Mathew, K.; Kolluru, V. S. C.; Hennig, R. G. VASPsol: Implicit solvation and

electrolyte model for density-functional theory. https://github.com/henniggroup/VASPsol, 2018; https://github.com/henniggroup/VASPsol.

() Mathew, K.; Sundararaman, R.; Letchworth-Weaver, K.; Arias, T. A.; Hennig, R. G. Implicit solvation model for density-functional study of nanocrystal surfaces and reaction pathways. *J. Chem. Phys.* **2014**, *140*, 084106.

() Mathew, K.; Kolluru, V. S. C.; Mula, S.; Steinmann, S. N.; Hennig, R. G. Implicit self-consistent electrolyte model in plane-wave density-functional theory. *J. Chem. Phys.* **2019**, *151*, 234101.

() Kohn, W.; Sham, L. J. Self-Consistent Equations Including Exchange and Correlation Effects. *Phys. Rev.* **1965**, *140*, A1133–A1138.

() Hammer, B.; Hansen, L. B.; Nørskov, J. K. Improved adsorption energetics within density-functional theory using revised Perdew-Burke-Ernzerhof functionals. *Phys. Rev. B* **1999**, *59*, 7413–7421.

() Blöchl, P. E. Projector augmented-wave method. *Phys. Rev. B* **1994**, *50*, 17953–17979.

() Monkhorst, H. J.; Pack, J. D. Special points for Brillouin-zone integrations. *Phys. Rev. B* **1976**, *13*, 5188–5192.

() Pack, J. D.; Monkhorst, H. J. "Special points for Brillouin-zone integrations"—a reply. *Phys. Rev. B* **1977**, *16*, 1748–1749.

() Nørskov, J. K.; Rossmeisl, J.; Logadottir, A.; Lindqvist, L.; Kitchin, J. R.; Bligaard, T.; Jónsson, H. Origin of the Overpotential for Oxygen Reduction at a Fuel-Cell Cathode. *The Journal of Physical Chemistry B* **2004**, *108*, 17886–17892.

() Rossmeisl, J.; Qu, Z.-W.; Zhu, H.; Kroes, G.-J.; Nørskov, J. Electrolysis of water on oxide surfaces. *Journal of Electroanalytical Chemistry* **2007**, *607*, 83–89, Theoretical and Computational Electrochemistry.

() Rossmeisl, J.; Logadottir, A.; Nørskov, J. Electrolysis of water on (oxidized) metal surfaces. *Chemical Physics* **2005**, *319*, 178–184, Molecular Charge Transfer in Condensed Media - from Physics and Chemistry to Biology and Nanoengineering in honour of Alexander M. Kuznetsov on his 65th birthday.

() Granda-Marulanda, L. P.; Rendón-Calle, A.; Builes, S.; Illas, F.; Koper, M. T. M.; Calle-Vallejo, F. A Semiempirical Method to Detect and Correct DFT-Based Gas-Phase Errors and Its Application in Electrocatalysis. *ACS Catalysis* **2020**, *10*, 6900–6907.

() Tang, M. T.; Liu, X.; Ji, Y.; Norskov, J. K.; Chan, K. Modeling Hydrogen Evolution Reaction Kinetics through Explicit Water–Metal Interfaces. *The Journal of Physical Chemistry C* **2020**, *124*, 28083–28092.
